# Supplementary material for: Quantum chaos in SU_3 models with trapped ions
Source: arXiv:1305.5141 source file (2013-07-23)
Supplement: Supplementary file 1 [file suppl-material.pdf]

# Supplementary Material to "Quantum chaos in $SU_3$ models with trapped ions"

Tobias Graß[1], Bruno Juliá-Díaz[1,2], Marek Kuś[3], Maciej Lewenstein[1,4]
[1]*ICFO-Institut de Ciències Fotòniques, Parc Mediterrani de la Tecnologia, 08860 Barcelona, Spain*
[2] *Departament d'Estructura i Constituents de la Matèria, Universitat de Barcelona, 08028 Barcelona, Spain*
[3] *Center for Theoretical Physics, Polish Academy of Sciences Al. Lotnikow 32/46, 02-668 Warszawa, Poland and*
[4] *ICREA - Institució Catalana de Recerca i Estudis Avançats, 08010 Barcelona, Spain*

## FIDELITY OF THE QUANTUM SIMULATION OF THE LMG MODEL

In the main text of the article we show that the dynamics of the trapped ions is given by the Hamiltonian

$$H_{\rm spin} = H_{\rm B} + H_{\rm J} \equiv H_{\rm B} + \sum_{\alpha} \sum_{m \leq m'}^{N} J_{\alpha}^{(m,m')} \tau_{\alpha}^{(m)} \tau_{\alpha}^{(m')}, \tag{1}$$

where $H_{\rm B}$ is a magnetic field term, and $H_{\rm J}$ a spin-spin interaction. The coupling strengths $J_{\alpha}^{(m,m')}$ are given in terms of the vibrational matrix $\mathcal{K}$ (see main text for a definition), which is diagonalized by the eigenmodes. A beat note $\mu_\alpha$ of the Raman coupling can be used to tune the transition closer to a resonance with one particular eigenmode than with the others. In that way, the form of $J_{\alpha}^{(m,m')}$ can be tuned, and, if the contribution from the center-of-mass mode is dominant, the coupling $J_{\alpha}^{(m,m')}$ will be approximately the same for all pairs $m$ and $m'$. We have shown in the main text that in this limit the Hamiltonian of Eq. (1) becomes equivalent to the LMG Hamiltonian. Explicitly, this "ideal" Hamiltonian reads:

$$H_{\rm ideal} = \frac{B}{\sqrt{2}}(\tilde{S}_{11} - \tilde{S}_{33}) + J \sum_{\sigma<\sigma'} \tilde{S}_{\sigma\sigma'} \tilde{S}_{\sigma\sigma'}. \tag{2}$$

It is thus argued that the ion setup allows for simulating this model, which has interesting dynamical behavior between chaos and regular motion. In this supplementary material, we investigate the fidelity of such a quantum simulation.

The proposed setup contains three systematic sources of error:
(i) The spin dynamics is not exactly given by Eq. (1), but is also influenced by a residual spin-phonon coupling, denoted by $\phi_\alpha$ in Eq. (3) of the main text, and oscillatory terms in Eq. (3) and Eq. (5) of the main text. (ii) Experimental imperfections, heating, and dephasing (e.g. by spontaneous emission), reduce the fidelity of the simulation. (iii) The spin part of Eq. (1) is not precisely the LMG model due to inevitable spatial dependencies of the coupling constant $J_{\alpha}^{(i,j)}$.

The first and second concerns, (i) and (ii), apply to all spin model simulations with trapped ions. The influence of the residual terms has been analyzed in Ref. [1]. The error for each coupling $\alpha$ can be approximated by $E \approx 4(1+\bar{n})\eta^2 \approx 8(1+\bar{n})\frac{J_\alpha \delta_\alpha \omega_\alpha^2}{\Omega_\alpha^2 \omega_0}$. For a typical equilibrium distance of $d = 2\mu$m and Yb$^+$, $\omega_0$ is of the order of 5MHz. To avoid zig-zag deformations of the ion chain, the trapping frequency has to be of the same order or larger [2]. We fix it to $\omega_\alpha = 0.1\omega_0/\delta_\alpha$, and choose a beat note detuning of $\delta_\alpha \leq 0.1$. Then the error $E$ for each coupling is 0.01, at coupling strength of the order $J_\alpha = 10\delta_\alpha$kHz, if we choose Rabi frequencies $\Omega$ of 1MHz, and cool the system to a mean phonon number $\bar{n} = 1.5$.

Under these circumstances, imperfections of type (ii) are expected to be a major source of errors. As they accumulate with time, the duration of a quantum simulation is restricted to a few milliseconds. In this context, it is thus important to ask whether the quantum dynamics we propose to observe happens on that time scale. The observable in Fig. 3 (b,c) is the spin population as a function with time, in time scales given by $J^{-1}$. With the value estimated above, the time scale is thus set to milliseconds which is within experimentally feasible scales. Certainly, the amount of type (ii) errors will also depend on the size of the system. As discussed in [3], increasing the number of particles has the strongest effect on the spontaneous emission rates due to the carrier transition simulating the $B$ field. Here, the errors will grow as $N^{1/3}$, which will set some limitations to the maximum size of the system. On the other hand, from a comparison of the dynamics shown in Fig. 3 (b,c) of the main text for different system sizes ($N = 4, 6$ and 8), we find that the time scale of the fast spin oscillations remains unchanged, while the envelope of the oscillations gains contributions of higher frequencies when the system size is increased. Since it is this envelope which distinguishes regular motion from chaotic one, a distinction should be possible on shorter time scales for larger systems.

Finally, the third error, (iii), is specific for quantum simulations of infinite-range interactions [3]. The error is zero in the limit $\delta_\alpha \to 0$, but this choice is incompatible with finite errors of type (i). In practice, one has to make $\delta_\alpha$ small enough to have small type (iii) errors, and at the same time large enough to have, for a given coupling strength $J$, sufficiently small type (i) errors.

We have studied the influence of $\delta_\alpha$ on the fidelity of the quantum simulation for trapping frequencies $\omega_\alpha = 0.1\omega_0/\delta_\alpha$ in the range $0.1 \leq \delta_\alpha \leq 1$, where $\delta_\alpha = 1$ corresponds to a Raman coupling without beat note. The results for $N = 4$ and $N = 8$ are shown in Fig. 1(a): Up to a critical trap frequency (which decreases with system size) the overlap between the ground state of the realistic

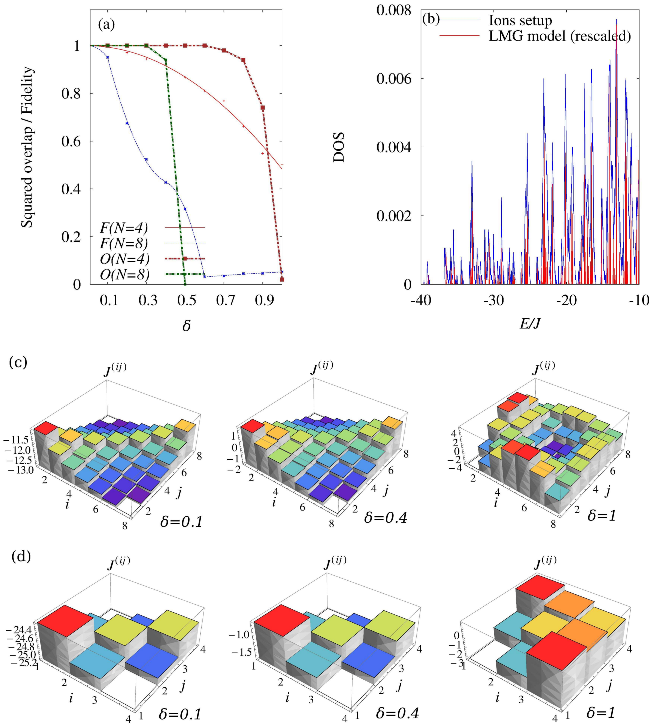


FIG. 1. (Color online) (a) For $N = 4$ ($N = 8$), the squared overlap between the ground state of the ion simulation ($H_{\text{spin}}$) and the LMG model ($H_{\text{ideal}}$) is shown as a function of the relative beat note detuning $\delta_\alpha$. We also show the overlap of a space spanned by the 15 (45) most symmetric eigenstates of $H_{\text{spin}}$ and the fully symmetric subspace. (b) The spectral density of the ion simulation and the LMG model are compared in the subspace of even parity and *eee* signature class for $N = 10$ (7503 states). The position-dependent interactions in the ion setup wash out the spectral peaks of the ideal model, which have been brought to a comparable height by rescaling them with a factor $1/N$. We also have slightly shifted energies by $\Delta E/J = 0.2$. (c,d) For $N = 8$ and $N = 4$, we illustrate the values of the coupling constants in the ion simulation for different beat note detunings $\delta_\alpha$.

system, Eq. (1), and the ideal model, Eq. (2), is 1, but then quickly drops to zero. A similar behavior can be found with respect to other eigenstates at the low energy edge of the spectrum. This behavior is understood from the coupling constants $J^{(i,j)}$ shown in Fig. 1(c,d) for different, specific choices of $\delta_\alpha$. While a sufficiently small value of $\delta_\alpha$, for any $N$ yields the quasi-infinite range behavior, the coupling constant stronly depends on $i$ and $j$ for larger $\delta_\alpha$.

For the dynamics of the system, the whole spectrum may play a role. In Fig. 1(b), we have therefore plotted the density of states (DOS) of the ideal and the realistic system with $N = 10$ and at $\delta_\alpha = 0.1$. The peaks occur at almost the same energies, but the realistic interactions broaden the peaks. In particular, states belonging to different spin symmetries (that is Young tableaux) appear degenerate in the ideal system, whereas the realistic model breaks this symmetry and thereby lifts these degeneracies.

It is thus interesting to ask with which fidelity an initial state with a well-defined spin symmetry will remain in the corresponding Hilbert space. Focusing on the fully symmetric spin configurations, we estimate this fidelity by calculating the overlap between the $D$-dimensional fully symmetric subspace and the $D$ most symmetric eigenstates of the realistic system. As plotted in 1(a), for $N = 4$ ($D = 15$) this fidelity is larger than 0.95 for up to $\delta_\alpha \approx 0.25$. For $N = 8$ ($D = 45$), we achieve an equally large fidelity still for $\delta_\alpha \approx 0.1$. Note that in this analysis, we have only taken into account the interaction term of Eqs. (1) and (2). The additional presence of a magnetic field term, $H_{\text{B}}$, being identical in both the ideal and the realistic model, would obviously increase fidelities (up to 1) in the limit of $B/J \to \infty$.

Our observations from Fig. 1(a) show that it is impossible to keep the errors of type (iii) on a constant level while increasing the particle number $N$, unless one decreases $\delta_\alpha$. In fact, as the bandwith of the vibrational spectrum does not change with $N$, and thus the energy difference between different modes scales with $1/N$, we have to rescale $\delta_\alpha$ by the same factor $1/N$ [3]. In this case, both, errors of type (i) and the coupling constant, remain unchanged by this re-scaling if one simultaneously decreases the Rabi frequencies by a factor $1/\sqrt{N}$.

---

[1] D. Porras and J. I. Cirac, Phys. Rev. Lett. **92**, 207901 (2004).
[2] D. H. E. Dubin and T. M. O'Neil, Rev. Mod. Phys. **71**, 87 (1999).
[3] K. Kim, M. S. Chang, S. Korenblit, R. Islam, E. E. Edwards, J. K. Freericks, G. D. Lin, L. M. Duan, and C. Monroe, Nature **465**, 590 (2010).
